# Supplementary material for: Seeing and Hearing: Open-domain Visual-Audio Generation with Diffusion Latent Aligners
Source: arXiv:2402.17723 source file (2024-02-27)
Supplement: Supplementary file 1 [file X_suppl.tex]

\clearpage
\setcounter{page}{1}
\maketitlesupplementary

\section{Hyper parameters}
% hyper-parameters 
% lr, inf_steps, num_optim_steps, clip_duration, clips_per_video, optimization_starting_point, ramdom_seed 
We provide the hyper-parameters as Table~\ref{table:hyper}. In the table, \textit{Lr} means learning rate; \textit{Inf\_steps} means the number of diffusion denoising steps; \textit{num\_optim\_steps} means the number of optimization steps per diffusion denoising step; \textit{optim\_start} means the starting point to perform optimization, i.e., 0.2 means start the optimization at diffusion step 6; \textit{seed} means the random seed for our experiments. 
\begin{table}[h]
\begin{tabular}{lllll}
\hline
Parameter              & V2A & A2V & I2A & Joint VA \\ \hline
Lr                & 0.1            & 0.01           & 0.1            & 0.01\&0.1         \\
Inf\_steps        & 30             & 30             & 30             & 30                \\
num\_optim\_steps & 1              & 1              & 1              & 1                 \\
optim\_start      & 0.2            & 0              & 0.2            & 0                 \\
seed              & 33             & 33             & 33             & 33                \\ \hline
\end{tabular}
\caption{Hyper-parameters for our tasks.}
\label{table:hyper}
\end{table}

\section{Supplementary video}
For further results, we refer the reader to our supplementary video, which presents the results of our method on the video-to-audio, audio-to-video, and joint audio-video generation tasks. 
For the video-to-audio task, our method can clearly generate better audio that aligns with the input video than the SpecVQGAN~\cite{iashin2021specvqgan}. For the audio-to-video generation task, our generated videos have higher visual quality and better alignment with the input audio than the baseline TempoToken~\cite{yariv2023tempotokens}. For the joint audio-video generation task, our method can produce both higher visual quality on video generation and better audio quality on audio generation than MM-Diffusion~\cite{ruan2023mm}. Moreover, our method takes text prompts as a condition and thus provides users more control for the generated contents.
